# Supplementary material for: Master Graduation Thesis: A Lightweight and Distributed Container-based Framework
Source: arXiv:2108.03562 source file (2021-08-08)
Supplement: Supplementary file 1 [file AppendixA.tex]

\chapter{An Appendix}
